# Supplementary material for: Neural Program Generation Modulo Static Analysis
Source: arXiv:2111.01633 source file (2021-11-22)
Supplement: Supplementary file 1 [file Supplementary.tex]

% REFER to main.py for all the include stmts

% \input{additional_examples}

% \input{SemConsistency}

% % \noindent \textbf{Data Extraction}:
% % \newpage

% \input{transformer_details}
