# Supplementary material for: Neural Program Generation Modulo Static Analysis
Source: arXiv:2111.01633 source file (2021-11-22)
Supplement: Supplementary file 2 [file design_nag.tex]

\section{Example: Designing a \nag}\label{appendix:design}

The design principles outlined in Section \ref{sec:condproggen}
are best illustrated by considering a subset of a \nag for generating Java method bodies.
Consider generating the body of the method discussed in Sect.\ \ref{sec:overview}:

\begin{codesmall2}
void write(File f, String str) {} 
\end{codesmall2}

Consider the following (partial) attribute grammar for a \nag that generates Java programs:\footnote{\label{footnote:MethodInvocationSynthesisOrder}Note that while this attribute grammar requires $\symb{Method}$ to be expanded before $\symb{Expr}$ (as inherited attributes of the latter depend on synthesized attributes of the former), the grammar is still $L$-attributed if we expand $\symb{Method}$ then $\symb{Expr}$ and perform a re-write trick to output the subtree produced by $\symb{Expr}$ first.} 
\[
\begin{array}{r@{\hspace{0.5ex}}c@{\hspace{2.0ex}}l}
  \symb{Start} & : & \symb{Stmt}\textbf{;}~[ \\
                % &&
                % \symb{Start}.\att{symTab}\downarrow~:=~\{\}\downarrow~  \\
                &&
             \symb{Stmt}.\att{symTab}\downarrow~:=~\symb{Start}.\att{symTab}\downarrow;~ ] \\ \\
  \symb{Stmt} & : & \symb{Stmt}\textbf{;}~\symb{Stmt}\textbf{;}~[ \\
                &&  \symb{Stmt}\$1.\att{symTab}\downarrow~:=~\symb{Stmt}\$0.\att{symTab}\downarrow ;\\ 
                &&  \symb{Stmt}\$2.\att{symTab}\downarrow~:=~\symb{Stmt}\$1.\att{symTabOut}\uparrow; \\ 
                &&  \symb{Stmt}\$0.\att{symTabOut}\uparrow~:=~\symb{Stmt}\$2.\att{symTabOut}\uparrow;~] \\ \\
  \symb{Stmt}  & : &
  \symb{Expr}~\textbf{.}~\symb{Method}~\textbf{(}\symb{ArgList}\textbf{)}~[ \\
              &&   
            \symb{Method}.\att{symTab}\downarrow~:=~\symb{Stmt}.\att{symTab}\downarrow; \\ 
             &&   
            \symb{Expr}.\att{type}\downarrow~:=~\symb{Method}.\att{callerType}\uparrow; \\
              &&   
              \symb{Expr}.\att{symTab}\downarrow~:=~\symb{Stmt}.\att{symTab}\downarrow; \\
              &&   
              \symb{ArgList}.\att{typeList}\downarrow~:=~\symb{Method}.\att{typeList}\uparrow ;\\
              &&   
              \symb{ArgList}.\att{symTab}\downarrow~:=~\symb{Stmt}.\att{symTab}\downarrow ;\\
              &&   
              \symb{Stmt}.\att{symTabOut}\uparrow~:=~\symb{Stmt}.\att{symTab}\downarrow;~]\\
        & \mid & \symb{DeclType}~\symb{Var}~\textbf{=}~\textbf{new}~\symb{NewType}~\textbf{(}\symb{ArgList}\textbf{)}~[ \\
           &&   
              \symb{DeclType}.\att{symTab}\downarrow~:=~\symb{Stmt}.\att{symTab}\downarrow;\\
           &&   
              \symb{Var}.\att{symTab}\downarrow~:=~\symb{Stmt}.\att{symTab}\downarrow;\\
           &&   
              \symb{ArgList}.\att{typeList}\downarrow~:=~\symb{NewType}.\att{typeList}\uparrow ;\\
           &&   
              \symb{NewType}.\att{declType}\downarrow~:=~\symb{DeclType}.\att{type}\uparrow;\\
           &&   
              \symb{ArgList}.\att{symTab}\downarrow~:=~\symb{Stmt}.\att{symTab}\downarrow ;\\
           &&   
              \symb{Stmt}.\att{symTabOut}\uparrow~:=~\symb{Stmt}.\att{symTab}\downarrow + \\
           &&  
              \quad (\symb{Var}.\att{name}\uparrow~\mapsto~\symb{DeclType}.\att{type}\uparrow);~]
\end{array}
\]

% \twr{Need to clean up w.r.t.\ $\symb{Start}$, $\symb{Goal}$, $\symb{ProcBody}$, and $\symb{Stmt}$.} \\
% \twr{Note that I have changed the left-hand-side nonterminal to $\symb{Stmt}$, which is what one would normally have in a programming-language grammar;
% however, the $\symb{Goal}$ nonterminal for this example is $\symb{ProcBody}$.}\\
% \rohan{The explanation below requires us to have some notion of $\symb{Start}$ to take the context into account. I added an extra rule in the grammar for that $\symb{Start} : \symb{Stmt}$ } \\
% \dc{Shouldn't the third line in the above equation be $\symb{Stmt}\$2.\att{symTab}\downarrow~:=~\symb{Stmt}\$1.\att{symTabOut}\uparrow$?} \\
% \rohan{Correct, has been resolved} \\

% To generate the body of \texttt{write}, we must first select an RHS for the $\symb{Start}$ symbol.

Synthesis using the \nag begins by extracting the context $\sX$ around the \texttt{write} method, and using this information to sample $\sZ$ from $P(Z | \sX)$.
Next, a Java compiler processes the surrounding code to form the attributes $A(\symb{Start}){\downarrow}$, which in our example takes the form of a symbol table:
\[
    \{~ \texttt{f} \mapsto \texttt{File},
    \texttt{str} \mapsto \texttt{String} ~\} \nonumber
\]

Producing a program from the \nag based upon this attribute grammar is done by first sampling from the distribution $P(\symb{Start} | \langle \rangle, A(\symb{Start}){\downarrow}, \sZ)$.
Because there is only one possible RHS for $\symb{Start}$ in our example, it is expanded to ``$\symb{Stmt}\textbf{;}$''.
% ``$\symb{Stmt}\textbf{;}\textrm{ }\symb{Stmt}\textbf{;}$''. 

Expanding the first $\symb{Stmt}$, the \nag needs to choose between a method invocation and a variable declaration. 
Because the \nag is ``aware'' that this step is to expand the first line of the method---the list of RHS values chosen so far is empty---we may expect it is perhaps likely to declare a variable.
This choice gives us the RHS  ``$\symb{DeclType}~\symb{Var}~\textbf{=}~\textbf{new}~\symb{NewType}~\textbf{(}\symb{ArgList}\textbf{)}$''. Expanding $\symb{DeclType}$, the \nag samples a Java type from the distribution 
\begin{align}
P(&\symb{DeclType} | \langle\textrm{``}\symb{Stmt}\textbf{;}~\symb{Stmt}\textbf{;}\textrm{''}, \textrm{``}\symb{DeclType}~\symb{Var}~\textbf{=}\nonumber \\ &\textbf{new}~\symb{NewType}~\textbf{(}\symb{ArgList}\textbf{)}\textrm{''} \rangle, A(\symb{DeclType}){\downarrow}, \sZ). \nonumber
\end{align}
Let us assume that the rules for expanding $\symb{DeclType}$ are:
\[
\begin{array}{r@{\hspace{0.5ex}}c@{\hspace{2.0ex}}l}
  \symb{DeclType} & : & \textbf{String}~[ \\
           &&   \symb{DeclType}.\att{type}\uparrow ~:=~\textbf{String};~]\\
           & \mid & \textbf{FileWriter}~[\\
            &&   \symb{DeclType}.\att{type}\uparrow ~:=~\textbf{FileWriter};~]\\
           & \mid & ...
\end{array}
\]
Thus, the \nag can choose any Java type as the declared type of the variable. At this point, the \nag has access to a significant amount of information to make the choice:
it is aware that the goal is to create a method called \texttt{write} (this is encoded in $\sZ$);
it is aware that it is choosing a type to be declared on the first line of the method;
and it has access to the symbol table that is maintained as part of $A(\symb{DeclType}){\downarrow}$.  Thus, the \nag may decide to expand the symbol $\symb{DeclType}$ to \texttt{FileWriter}. This type is then passed upward via the synthesized attribute $\symb{DeclType}.\att{type}{\uparrow}$.  

Next, the grammar must expand the $\symb{Var}$ rule and pick a variable name to declare:
\[
\begin{array}{r@{\hspace{0.5ex}}c@{\hspace{2.0ex}}l}
   \symb{Var}     & : & \textbf{var\_0}~[\\
              &&   
              \symb{Var}.\att{name}\uparrow~:=~\textbf{var\_0}];~] \\ 
           & \mid & \textbf{var\_1}~[\\
              &&   
              \symb{Var}.\att{name}\uparrow~:=~\textbf{var\_1}];~] \\
           & \mid & ...
\end{array}
\]
This choice is returned via the synthesized attribute  $\symb{Var}.\att{name}{\uparrow}$. Now it is time to expand $\symb{NewType}$:
\[
\begin{array}{r@{\hspace{0.5ex}}c@{\hspace{2.0ex}}l}
  \symb{NewType} & : & \textbf{String}~[ \\
           && \symb{NewType}.\att{typeList}\uparrow ~:=~\langle \textbf{char[]}, \textbf{String} \rangle ;~]\\
           & \mid & \textbf{FileWriter}~[\\
            && \symb{NewType}.\att{typeList}\uparrow ~:=~\langle \textbf{File} \rangle ;~]\\
           & \mid & ...
\end{array}
\]
Here is where the attributes make things easier: when sampling from $P(\symb{NewType} | ...)$, the \nag has access to $\symb{NewType}.\att{type}{\downarrow}$, which takes the value \texttt{FileWriter}. A synthesizer may err by choosing a type that is not compatible with \texttt{FileWriter}.  However, we may expect that during training, every time that $\symb{NewType}$ was expanded and the declared type was \texttt{FileWriter}, the type chosen was either \texttt{FileWriter} or some subclass of \texttt{FileWriter}, and hence the \nag is unlikely to make an error.  Without the attributes, a simple conditional neural grammar must learn to remember the declared type and its importance to choosing the RHS for $\symb{NewType}$, whereas the \nag is explicitly presented with it.
Consequently, the \nag has a significant advantage.  

Assume that the \nag chooses \texttt{FileWriter}. It must now expand the $\symb{ArgList}$ symbol:
\[
\begin{array}{r@{\hspace{0.5ex}}c@{\hspace{2.0ex}}l}
  \symb{ArgList}    & : &  \symb{Var}~\textbf{,}~\symb{Var}~\textbf{,}~\textbf{...}~\textbf{,}~\symb{Var}~[\\
           &&  
              \symb{Var}\$0.\att{expType}\downarrow~:=~\symb{ArgList}.\att{typeList}\downarrow[0];\\
           && 
              \symb{Var}\$0.\att{symTab}\downarrow~:=~\symb{ArgList}.\att{symTab}\downarrow;\\
           &&  
              \symb{Var}\$1.\att{expType}\downarrow~:=~\symb{ArgList}.\att{typeList}\downarrow[1];\\
           &&  
              \symb{Var}\$1.\att{symTab}\downarrow~:=~\symb{ArgList}.\att{symTab}\downarrow~...;~] \\ \\
  \symb{Var}     & : & \textbf{var\_0}~[\\
              &&  
              \symb{Var}.\att{type}\uparrow~:=~\symb{Var}.\att{symTab}\downarrow[\textbf{var\_0}];~] \\ 
           & \mid & \textbf{var\_1}~[\\
              &&  
              \symb{Var}.\att{type}\uparrow~:=~\symb{Var}.\att{symTab}\downarrow[\textbf{var\_1}];~] \\
           & \mid & ...
\end{array}
\]
Again the \nag has a significant advantage over a CNG, because the \nag has access to $\symb{ArgList}.\att{typeList}{\downarrow}$ (an explicit representation of the types required by the constructor being called) and, most importantly, $\symb{ArgList}.\att{symTab}{\downarrow}$.  
Thus, the \nag has access to an explicit list of the variables in scope, as well as their types.  At this point, it is an easy matter for the \nag to match the required type of the first argument to the constructor (\texttt{File}) with an appropriate variable in the symbol table (\texttt{f}).  
Contrast this with a CNG, which would have had to somehow learn to ``remember'' the variable \texttt{f} and its type when generating $\sZ$ from $P(Z | \sX)$ (assuming that \texttt{f} was encoded as part of the evidence set $\sX$).

Now that the declaration of \texttt{var\_0} has been fully expanded, the \nag contains a rule for updating the symbol table and adding the newly-declared variable \texttt{var\_0}, and the attribute $\symb{Stmt}.\att{symTab}{\uparrow}$ takes the value:
\begin{align}
    \{ \texttt{f} &\mapsto \texttt{File}, \nonumber \\
    \texttt{str} &\mapsto \texttt{String}, \nonumber \\
    \texttt{var\_0} &\mapsto \texttt{FileWriter} \} \nonumber
\end{align}
When the second right-hand side $\symb{Stmt}$ symbol is expanded, the symbol table is passed down via the inherited attribute $\symb{Stmt}\$1.\att{symTab}\downarrow$.
All of the information available---the latent variable $\sZ$ encoding the contextual information (including the name of the method ``\texttt{write}'' being generated), and the symbol table containing a \texttt{FileWriter} and a \texttt{String})---helps the \nag to deduce correctly that this $\symb{Stmt}$ symbol should be expanded into a method invocation that calls \texttt{write}.
Furthermore, the presence of the symbol table makes it easy for the \nag to correctly attach the \texttt{write} method call to the variable \texttt{var\_0}, and to use \texttt{str} as the argument.
